# Supplementary material for: Dense2MoE: Restructuring Diffusion Transformer to MoE for Efficient Text-to-Image Generation
Source: arXiv:2510.09094 source file (2025-10-10)
Supplement: Supplementary file 1 [file X_suppl.tex]

\clearpage
\setcounter{page}{1}
\maketitlesupplementary

\section{Preliminary}
\label{appendix:preliminary}

\textbf{Diffusion Models.} 
% 3.1.1 Diffusion Models, SDE, RFs
Diffusion models (DMs)~\cite{ho2020denoising} are a class of generative models that gradually add noise to the data and then learn to reverse this process to reconstruct the data. 
The forward process can be described by the following Stochastic Differential Equation (SDE)~\cite{song2021scorebased}:
\begin{equation}
\text{d}\mathbf{x}_t = \mathbf{f}(\mathbf{x}_t, t) \text{d}t + \mathbf{g}(t) \text{d}\mathbf{w}_t,
\end{equation}
where $\mathbf{x}_t$ represents the sample at time $t \in [0,1]$, $\mathbf{f}(\mathbf{x}_t, t)$ is the drift term, $\mathbf{g}(t)$ is the diffusion coefficient, and $\mathbf{w}_t$ is the Wiener process.
The SDE is proved to have the same solution trajectories as the Probability Flow (PF) ODE.
Let $p(\mathbf{x}_t)$ denote the data distribution at time $t$, $p(\mathbf{x}_0)$ the empirical data distribution, and $p(\mathbf{x}_1)$ the prior distribution, the ODE reverse process is formulated as
\begin{equation}
\text{d}\mathbf{x}_t = [\mathbf{f}(\mathbf{x}_t, t) - \frac12\mathbf{g}^2(t) \nabla_{\mathbf{x}_t} \log p(\mathbf{x}_t)] \text{d}t,
\end{equation}
where $\nabla_{\mathbf{x}_t} \log p(\mathbf{x}_t)$ represents the gradient of the log-likelihood of the data distribution, referred to as the score function. 
Diffusion models estimate this score function through a trainable neural network $s_{\theta}(\mathbf{x}, t)$.  

As a variant of DMs, Rectified Flows (RFs)~\cite{liu2022flow} define the forward process as straight paths between $p(\mathbf{x}_0)$ and $p(\mathbf{x}_1)$, described by
\begin{equation}
\mathbf{x}_t = (1 - t) \mathbf{x}_0 + t \epsilon,
\end{equation}
where $\mathbf{x}_0 \sim p(\mathbf{x}_0)$ is the sampled data and $\epsilon \sim p(\mathbf{x}_1)$ is the Gaussian noise. 
In RFs, the network output directly parameterizes the velocity $v_{\theta}$, the objective is 
\begin{equation}
\mathcal{L} = \mathbb{E}_{\mathbf{x}_0 \sim p(\mathbf{x}_0), \mathbf{x}_1 \sim p(\mathbf{x}_1)}||v_{\theta}(\mathbf{x}_t, t) - (\mathbf{x}_1 - \mathbf{x}_0)||^2.
\end{equation}
RFs simply straighten the diffusion trajectory, facilitating efficient training and sampling.
\\[0.5em]
\textbf{Diffusion Transformer (DiT).}
Diffusion transformer~\cite{peebles2023scalable} is a diffusion backbone that exhibits excellent scaling properties.
It divides the image latent into patches and encodes them as tokens before being processed through multiple transformer blocks.
In DiT, a series of stacked blocks are used to learn hierarchical representations. Based on DiT, multimodal diffusion transformer (MMDiT)~\cite{esser2024scaling} extends the architecture to handle diverse data modalities by modality-specific attention projection and MLP layers for text and image. They only interact during the computation of the self-attention. The modality-specific design maintains the independence of different modality features.

FLUX.1 [dev] adopts a hybrid architecture for DiTs, comprising one-third double stream blocks (i.e., MMDiT blocks) and two-thirds single stream blocks, as shown in Fig.~\ref{fig:framework}.
Unlike double stream blocks, single stream blocks share all the layers for both text and image inputs, enabling efficient multi-modal fusion. 
With 19 double stream blocks and 38 single stream blocks, the 12B FLUX.1 [dev] model represents the state-of-the-art among open-source text-to-image models.
\begin{figure}[h]
\includegraphics[width=1.0\linewidth]{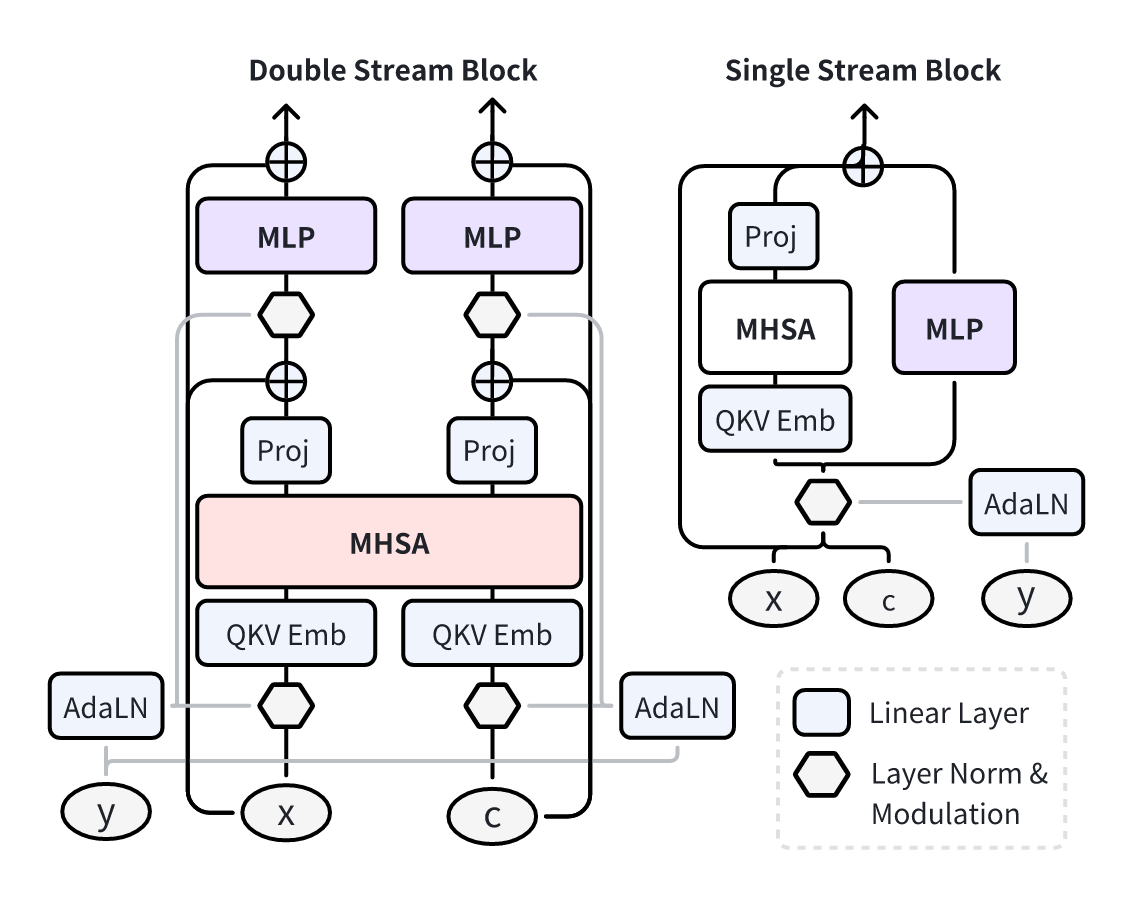}
\caption{Two kinds of Transformer blocks in FLUX.1}
\label{fig:block}
\end{figure}
\\[0.5em]

\begin{figure*}[h]
\hsize=\textwidth
\centering
\includegraphics[width=0.85\linewidth]{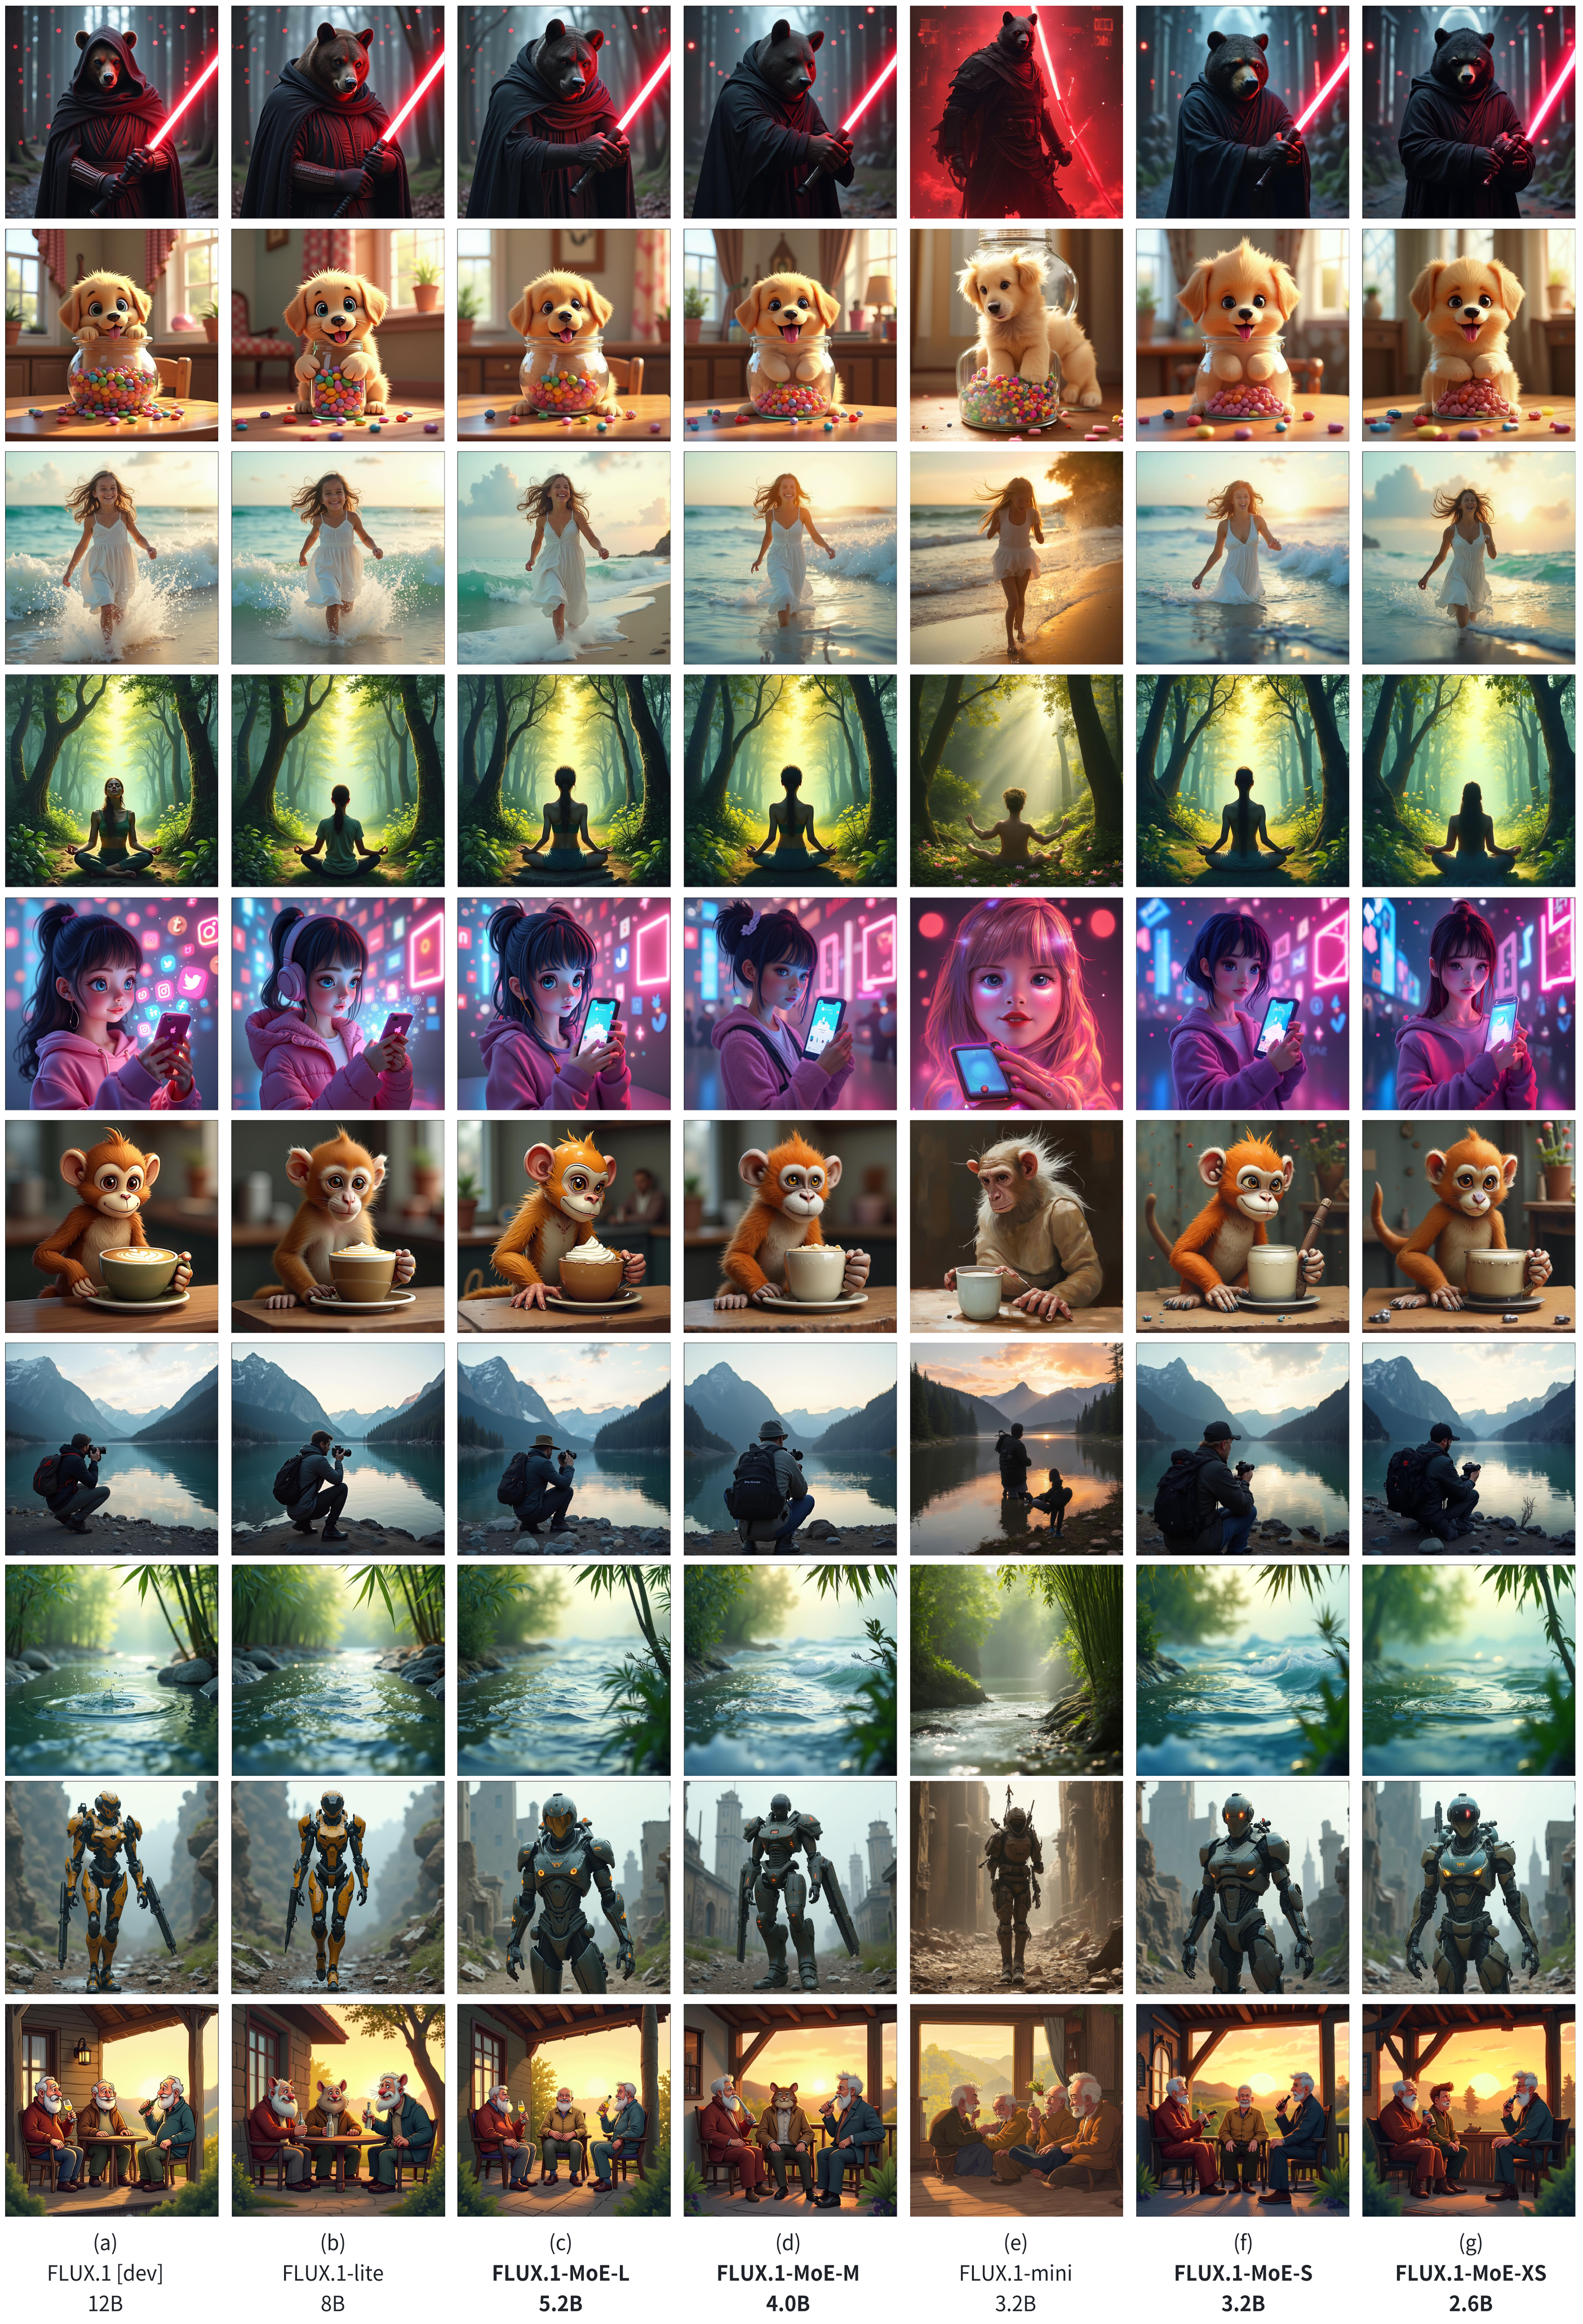}
\caption{The quantitative comparison includes FLUX.1-MoE models alongside the original FLUX.1 [dev] and pruning baselines, FLUX-Lite and FLUX-Mini. All images are generated using the same random noise.}
\label{fig:quantitative}
\end{figure*}

\section{Quantitative Comparison}
We present a quantitative comparison of ours FLUX.1-MoE models with the FLUX.1 [dev] model, as well as the pruned models FLUX-Lite (8B) and FLUX-Mini (3.2B) in Fig.~\ref{fig:quantitative}. 
The images show that excessive pruning, such as in FLUX-Mini (e), leads to significant degradation, with the model diverging further from the original. In contrast, at the same high activation parameter compression ratio, the Dense-to-MoE approach effectively preserves performance.
